# Supplementary material for: Federated Learning in ASR: Not as Easy as You Think
Source: arXiv:2109.15108 source file (2021-09-30)
Supplement: Supplementary file 1 [file appendix.tex]

\section*{Appendix}
\subsection*{Dataset Details}

In order to make the underlying Librispeech corpus\cite{librispeech} more suitable for a federated learning task we created new subsets from supersets of the conventional subsets.

Firstly, we define the superset of \texttt{test-clean} and \texttt{test-other} as \texttt{test} and the superset of \texttt{dev-clean} and \texttt{dev-other} as \texttt{dev}.
We combine all training-sets \texttt{train-clean-100}, \texttt{train-clean-360} and \texttt{train-other-500} into a \texttt{train} superset.

Secondly, we move all speakers with more than 116 utterances from \texttt{train}, \texttt{test} and \texttt{dev} to a set of simulated clients \texttt{FL}.
The remaining speakers are kept in their sets.
Those sets can be interpreted as server-side or secret sets, on which simulated clients have no access. 

Thirdly, we split the data of every speaker in \texttt{FL} into  60\% train-, 20\% test- und 20\% dev-subsets, which are referenced as \texttt{fl/ID/train}, \texttt{fl/ID/test} and \texttt{fl/ID/dev}, where \texttt{ID} represents a unique client identifier.

However, \texttt{train} has much more utterances than \texttt{fl/*/train}, where the star (*) indicates all speaker ids. For performance considerations, we decrease \texttt{train} to one third of \texttt{fl/*/train}, and denote this set as \texttt{initial/train}. The speakers in \texttt{initial/train} are used to train an initial model.

To analyse the performance in different speaker conditions, we manually create further development- and test-sets. Therefore, we move one utterance of each speaker from \texttt{dev} and \texttt{test} to \texttt{final/dev} and \texttt{final/test} sets. Since there is no speaker overlap between \texttt{initial/train}, \texttt{dev}, and \texttt{test}, we considered \texttt{final/dev} and \texttt{final/test} as unknown speaker sets. Then we move one utterance of every speaker from \texttt{initial/train} to either \texttt{final/pre-dev} or \texttt{final/pre-test} evenly. The same operation is also applied on \texttt{fl/*/train} to obtain \texttt{final/fl-dev} and \texttt{final/fl-test}.

Lastly, we create a superset \texttt{complete/train} from \texttt{fl/*/train} and \texttt{initial/train}. 
This superset will be used to generate an upper bound on the model performance.
The total amount of utterances can be found in Tab.~\ref{tab:utts}.
